# Supplementary material for: Towards Anatomically Plausible Human Image Generation via Synthetic Localized Preferences
Source: arXiv:2605.25759 source file (2026-11-25)
Supplement: Supplementary file 1 [file supplementary.tex]

\documentclass[runningheads]{llncs}

% ---------------------------------------------------------------
% Include basic ECCV package
 
% TODO REVIEW: Insert your submission number below by replacing '*****'
% TODO FINAL: Comment out the following line for the camera-ready version
\usepackage[review,year=2026,ID=658]{eccv}
% TODO FINAL: Un-comment the following line for the camera-ready version
%\usepackage{eccv}

% OPTIONAL: Un-comment the following line for a version which is easier to read
% on small portrait-orientation screens (e.g., mobile phones, or beside other windows)
%\usepackage[mobile]{eccv}

% ---------------------------------------------------------------
% Other packages

% Commonly used abbreviations (\eg, \ie, \etc, \cf, \etal, etc.)
\usepackage{eccvabbrv}

% Include other packages here, before hyperref.
\usepackage{graphicx}
\usepackage{booktabs}
\usepackage{tabularx}
\usepackage{tcolorbox}
\tcbuselibrary{listings}
\usepackage{float}

% The "axessiblity" package can be found at: https://ctan.org/pkg/axessibility?lang=en
\usepackage[accsupp]{axessibility}  % Improves PDF readability for those with disabilities.

% ---------------------------------------------------------------
% Hyperref package

% It is strongly recommended to use hyperref, especially for the review version.
% Please disable hyperref *only* if you encounter grave issues.
% hyperref with option pagebackref eases the reviewers' job, but should be disabled for the final version.
%
% If you comment hyperref and then uncomment it, you should delete
% main.aux before re-running LaTeX.
% (Or just hit 'q' on the first LaTeX run, let it finish, and you
%  should be clear).

% TODO FINAL: Comment out the following line for the camera-ready version
%\usepackage[pagebackref,breaklinks,colorlinks,citecolor=eccvblue]{hyperref}
% TODO FINAL: Un-comment the following line for the camera-ready version
\usepackage[pagebackref,breaklinks,colorlinks,citecolor=eccvblue]{hyperref}
\usepackage{wrapfig}

% Support for ORCID icon
\usepackage{orcidlink}

\usepackage{enumitem}

% colored authors
\definecolor{DeltaColor}{rgb}{0.039,0.73,0.71}
\definecolor{SigmaColor}{rgb}{0.98,0.45,0.0}
\definecolor{AlphaColor}{rgb}{0,0,0.8}
\definecolor{BetaColor}{rgb}{0.8,0,0.8}
\definecolor{GammaColor}{rgb}{0.514,0.34,0.224}
\definecolor{EpsilonColor}{rgb}{0.353,0.725,0.906}
\definecolor{PurpleColor}{HTML}{9839ff}
\definecolor{RedColor}{rgb}{0.949,0.275, 0.224}
\definecolor{citecolor}{HTML}{0071bc}

% author comments

% \renewcommand{\captionlabelfont}{\scriptsize}

\begin{document}

% ---------------------------------------------------------------
% TODO REVIEW: Replace with your title
\title{Supplementary Material for Towards Anatomically Plausible Human Image Generation via Synthetic Localized Preferences}

% TODO REVIEW: If the paper title is too long for the running head, you can set
% an abbreviated paper title here. If not, comment out.
\titlerunning{Abbreviated paper title}

% TODO FINAL: Replace with your author list. 
% Include the authors' OCRID for the camera-ready version, if at all possible.
\author{First Author\inst{1}\orcidlink{0000-1111-2222-3333} \and
Second Author\inst{2,3}\orcidlink{1111-2222-3333-4444} \and
Third Author\inst{3}\orcidlink{2222--3333-4444-5555}}

% TODO FINAL: Replace with an abbreviated list of authors.
\authorrunning{F.~Author et al.}
% First names are abbreviated in the running head.
% If there are more than two authors, 'et al.' is used.

% TODO FINAL: Replace with your institution list.
\institute{Princeton University, Princeton NJ 08544, USA \and
Springer Heidelberg, Tiergartenstr.~17, 69121 Heidelberg, Germany
\email{lncs@springer.com}\\
\url{http://www.springer.com/gp/computer-science/lncs} \and
ABC Institute, Rupert-Karls-University Heidelberg, Heidelberg, Germany\\
\email{\{abc,lncs\}@uni-heidelberg.de}}

\maketitle

\section{Implementation Details}
As introduced in Section 6.1 of the main paper, we use LoRA \cite{hu2022lora} with a rank of 32. All experiments are conducted on 8 NVIDIA A100 (80GB) GPUs. All images are processed at a resolution of $1024 \times 1024$.
For the optimization process, we employ the AdamW \cite{loshchilov2017decoupled} optimizer with a weight decay of 0.01. Both models are trained for 3,000 steps using an effective batch size of 16, accompanied by a linear learning rate warm-up of 200 steps.
Specifically for the FLUX \cite{flux2024} backbone, we apply a learning rate of $5e-6$, and set the spatial weighting scalar $\alpha = 10$ along with a regularization margin of $\tau = 0.01$ for our alignment objective. 
For SDXL \cite{rombach2022high} backbone, we apply a learning rate of $5e-5$, and set the spatial weighting scalar $\alpha = 10$ along with a regularization margin of $\tau = 0.002$ for our alignment objective.

\section{Details of HAF-Bench}
\subsection{Prompt Composition of HAF-Bench}
As introduced in Section 5 of the main paper, the HAF-Bench evaluation set comprises 500 rigorously curated prompts designed to evaluate the anatomical plausibility of generated human images. To ensure a comprehensive evaluation, the dataset is balanced across five distinct anatomical categories (100 prompts each), with each targeting a unique anatomical focus: (1) Basic Anatomy: Focuses on precise hand structure and numerical counting, (2) Semantic Gestures: Evaluates the generation of culturally recognizable hand signs, (3) Self-Interaction: Assesses realistic self-contact scenarios, (4) Object Interaction: Targets plausible hand-object manipulation, (5) Full Body: Examines anatomical plausibility in full-body shots. \cref{tab:haf_bench_prompts} showcases representative prompt examples for each category.

\begin{table}[H]
\centering
\caption{\textbf{Representative Prompts of the HAF-Bench Evaluation Set.} The benchmark comprises 500 challenging prompts evenly distributed across five distinct anatomical categories. Below we showcase representative examples for each category.}
\label{tab:haf_bench_prompts}

\vspace{-0.5em}

% Box 1: Basic Anatomy
\begin{tcolorbox}[colback=gray!5!white, colframe=gray!60!black, boxrule=0.5pt, arc=2pt, left=4pt, right=4pt, top=4pt, bottom=4pt, title=\footnotesize\textbf{1. Basic Anatomy} \hfill {Focus: Hand structure and numerical counting}]
\scriptsize
\textbullet~ A yoga instructor stretching her hand with an extended ring finger. \\
\textbullet~ A mother teaching her child to count to five with fingers. \\
\textbullet~ A little boy counting to ten, holding up both hands with all ten fingers spread.
\end{tcolorbox}
\vspace{-0.5em}

% Box 2: Semantic Gestures
\begin{tcolorbox}[colback=gray!5!white, colframe=gray!60!black, boxrule=0.5pt, arc=2pt, left=4pt, right=4pt, top=4pt, bottom=4pt, title=\footnotesize\textbf{2. Semantic Gestures} \hfill {Focus: Culturally recognizable hand signs}]
\scriptsize
\textbullet~ A man lying on the beach giving a relaxed thumbs-up. \\
\textbullet~ A nurse in scrubs making an OK gesture with slightly bent fingers in a hospital corridor. \\
\textbullet~ A girl in traditional hanbok making a single-hand finger heart with a shy smile.
\end{tcolorbox}
\vspace{-0.5em}

% Box 3: Self-Interaction
\begin{tcolorbox}[colback=gray!5!white, colframe=gray!60!black, boxrule=0.5pt, arc=2pt, left=4pt, right=4pt, top=4pt, bottom=4pt, title=\footnotesize\textbf{3. Self-Interaction} \hfill {Focus: Realistic self-contact scenarios}]
\scriptsize
\textbullet~ A child resting her chin on her hand with fingers slightly curved, daydreaming in a classroom. \\
\textbullet~ Two children holding hands tightly, fingers curled slightly, playing in a sunny park. \\
\textbullet~ Two friends laughing while gripping wrists with slightly bent fingers in a sunny park.
\end{tcolorbox}
\vspace{-0.5em}

% Box 4: Object Interaction
\begin{tcolorbox}[colback=gray!5!white, colframe=gray!60!black, boxrule=0.5pt, arc=2pt, left=4pt, right=4pt, top=4pt, bottom=4pt, title=\footnotesize\textbf{4. Object Interaction} \hfill {Focus: Plausible hand-object manipulation}]
\scriptsize
\textbullet~ A child holding a red apple with fingers wrapped around it. \\
\textbullet~ A woman holding a credit card between her thumb and index finger. \\
\textbullet~ A musician holding a guitar pick between two fingers.
\end{tcolorbox}
\vspace{-0.5em}

% Box 5: Full Body
\begin{tcolorbox}[colback=gray!5!white, colframe=gray!60!black, boxrule=0.5pt, arc=2pt, left=4pt, right=4pt, top=4pt, bottom=4pt, title=\footnotesize\textbf{5. Full Body} \hfill {Focus: Anatomical plausibility in full-body shots}]
\scriptsize
\textbullet~ A man sitting on a balcony full body, leaning his elbows on the railing and clasping his hands. \\
\textbullet~ A full body shot of a skateboarder carrying his board under one arm. \\
\textbullet~ A full body shot of a rock climber chalking their hands before a climb.
\end{tcolorbox}

\end{table}

\subsection{Agreement Between VLM and Human Perception}
As described in Section 5 of the main paper, to validate the reliability of Gemini-3-Pro \cite{google2025gemini3} as our automated visual judge, we conducted a comprehensive human evaluation on the generated samples. Human annotators were tasked with identifying anatomical errors under the same criteria used by the VLM.

Given a dataset of $N$ images, let $y_i^{Human} \in \{0, 1\}$ and $y_i^{VLM} \in \{0, 1\}$ denote the binary judgments (where $1$ indicates an anatomical error and $0$ indicates a plausible structure) from the human annotators and the VLM for the $i$-th image, respectively. The raw agreement rate is formulated as:
$$Agreement = \frac{1}{N} \sum_{i=1}^{N} \mathbb{I}(y_i^{VLM} = y_i^{Human})$$
where $\mathbb{I}(\cdot)$ is the indicator function. By comparing the paired judgments, we observed a high raw agreement rate of 82\%.

\begin{table}[H]
\centering
\caption{\textbf{System Prompt for VLM Evaluation.} The instruction prompt provided to Gemini-3-Pro for automated anatomical plausibility assessment.}
\label{tab:vlm_prompt}

\vspace{-0.5em}

\begin{tcolorbox}[colback=gray!5!white, colframe=gray!60!black, boxrule=0.5pt, arc=1pt, left=2pt, right=2pt, top=2pt, bottom=2pt, boxsep=1pt, fontupper=\scriptsize]

\noindent \textbf{*** ROLE ***} \\
You are a Senior Visual QA Specialist specializing in Human Anatomy. Your specific objective is to identify \textbf{Severe and Obvious} anatomical artifacts in AI-generated human images.

\vspace{0.3em}
\noindent \textbf{*** TASK ***} \\
Conduct a \textbf{general} anatomical plausibility check on the person(s) in the image. \textbf{PRIORITY FOCUS:} You must identify \textbf{glaring} errors in the \textbf{Face and Hands}.

\vspace{0.3em}
\noindent \textbf{CRITICAL TOLERANCE SETTINGS:}
\begin{enumerate}[leftmargin=*, noitemsep, topsep=0pt]
    \item \textbf{IGNORE} minor artifacts, artistic stylization, slight blur.
    \item \textbf{IGNORE} background characters or heavily occluded body parts.
    \item \textbf{ONLY FLAG} if the distortion is physically impossible and immediately visible. If unsure, result is "No".
\end{enumerate}

\vspace{0.3em}
\noindent \textbf{*** FAIL CRITERIA (WITH EXAMPLES) ***} \\
Analyze the image for the following defects. If ANY are found, the result is "Yes" (has distortion).

\vspace{0.3em}
\noindent \textbf{1. [HANDS \& FINGERS ISSUES]}
\begin{itemize}[leftmargin=*, noitemsep, topsep=0pt]
    \item \textbf{Obvious Polydactyly:} Explicitly visible extra fingers (e.g., 6+ fingers on one hand).
    \item \textbf{Unexplained Oligodactyly:} Fingers that are missing or cut off without cause. \\
    NOTE: Do NOT flag if fingers are hidden due to "Natural Occlusion" (e.g., holding an object, making a fist, blocked by perspective, or behind other body parts). Only flag if the hand structure itself is clearly incomplete.
    \item \textbf{Severe Malformation:} Fingers branching out incorrectly, "claw-like" distortion, or fingers looking like melted wax.
    \item \textbf{Fusion:} Syndactyly (fingers fused together without separation lines) or fingers merging into objects.
\end{itemize}

\vspace{0.3em}
\noindent \textbf{2. [FACE \& HEAD ISSUES]}
\begin{itemize}[leftmargin=*, noitemsep, topsep=0pt]
    \item \textbf{Severe Facial Collapse:} Features (eyes/nose/mouth) are mixed together, melted, or missing.
    \item \textbf{Gross Misplacement:} Eyes/ears appearing in the wrong position (e.g., eye on the cheek). \\
    NOTE: Do NOT flag for "Asymmetrical pupils" or "weird gaze" unless the eye is structurally broken.
\end{itemize}

\vspace{0.3em}
\noindent \textbf{3. [BODY \& LIMB ISSUES]}
\begin{itemize}[leftmargin=*, noitemsep, topsep=0pt]
    \item \textbf{Physiologically Impossible Joints:} Limbs bending backwards or arms attached at broken angles.
    \item \textbf{Surplus/Deficit:} Extra arms/legs appearing from behind, or limbs floating detached from the body.
    \item \textbf{Severe Blending:} Limbs melting indistinguishably into clothing or furniture.
\end{itemize}

\vspace{0.3em}
\noindent \textbf{*** OUTPUT RULES ***}
\begin{enumerate}[leftmargin=*, noitemsep, topsep=0pt]
    \item \textbf{CRITICAL:} Output ONLY the valid JSON string. Do NOT output any introductory text or markdown (like \texttt{```json}).
    \item The JSON must strictly contain two keys: "reasoning" (a step-by-step observation of the face, hands, and limbs) and "has\_distortion" ("Yes" or "No").
\end{enumerate}

\vspace{0.3em}
\noindent \textbf{*** OUTPUT EXAMPLES (Follow this exact format) ***} \\
Example 1 (Distortion found):
\{
"reasoning": "[Briefly describe the severe anatomical errors observed]", 
"has\_distortion": "Yes"
\}

Example 2 (No distortion found):
\{
"reasoning": "[Briefly describe why the structures are plausible]",
"has\_distortion": "No"
\}

\end{tcolorbox}
\end{table}

\section{Details of HAP Dataset}
\subsection{Visualization of Localized Degradation Mechanism}

\begin{figure}[!t]
  \centering
  \makebox[\textwidth][c]{\includegraphics[width=1.0\linewidth]{ECCV_2026_AnatomyDPO/figures/degradation.pdf}}
  \caption{\textbf{Extended Visualization of the HAP Dataset.} We showcase localized preference pairs targeting hand anomalies (top two rows) and facial degradations (bottom two rows). Positive samples (green boxes) display plausible anatomy, whereas synthesized negative samples (red boxes) exhibit explicit structural errors.
  }
  \label{fig:degradation}
\end{figure}

As introduced in Section 4.1 of the main paper, the foundation of the HAP dataset is built upon a localized degradation mechanism. This approach acts as a controlled experiment: it explicitly injects anatomical artifacts into highly articulated regions while keeping the global semantics, lighting, and background strictly identical. To better illustrate the quality, diversity, and strict control of these synthetic preference pairs, we provide an extended visualization in \cref{fig:degradation}.

\subsection{Details of Human Filtering Process}

The HAP dataset was curated from an initial candidate pool of approximately 25,000 synthesized preference pairs. A team of trained annotators conducted a manual filtering process on this raw pool. During the curation phase, annotators independently reviewed the image pairs and filtered out invalid data based on three strict criteria. Following this filtering process, 10,652 pairs (roughly 42.6\% of the raw pool) passed the quality checks to form the finalized dataset. The detailed filtering criteria are as follows:

\begin{itemize}[leftmargin=*, topsep=2pt, itemsep=2pt]
    \item \textbf{Criterion 1: High-Fidelity Positive Samples.} The positive image ($x_w$) must be anatomically accurate. Samples where the base generative model produced perceptible anatomical artifacts in the positive sample were discarded.
    \item \textbf{Criterion 2: Explicit Anatomical Degradation.} The negative sample ($x_l$) must present clearly visible anatomical errors. Samples exhibiting overly subtle artifacts or lacking explicit structural degradation were discarded.
    \item \textbf{Criterion 3: Strictly Preserved Background Compositions.} The non-targeted regions must remain strictly identical across the preference pair. Samples exhibiting noticeable background inconsistencies introduced by the localized degradation pipelines were discarded.
\end{itemize}

\section{Additional Ablation Study: Localized Weighting Mechanism}

An ablation study is conducted to evaluate the necessity of the localized weighting mechanism within the ASAP framework.
The proposed ASAP objective utilizes a spatial weighting scalar ($\alpha$) to explicitly concentrate the optimization signal on targeted anatomical regions. We compare the base FLUX model against a FLUX-ASAP variant trained entirely without this mechanism ($\alpha = 0$) in \cref{tab:ablation}.

\begin{table}[t]
    \centering
    \caption{  \textbf{Ablation on Localized Weighting Mechanism.} Quantitative evaluation of the spatial weighting scalar ($\alpha$) within the ASAP framework. Disabling the localized weighting ($\alpha=0$) significantly degrades anatomical alignment, evidenced by a higher Anatomical Error Rate (AER) and a lower Relative Success Index (RSI). Conversely, the complete FLUX-ASAP model ($\alpha=10$) achieves optimal anatomical correctness.}
    \label{tab:ablation}
    \resizebox{\linewidth}{!}{
    \begin{tabular}{l|cc|ccccc}
        \toprule
        \textbf{Models} & \textbf{AER} $\downarrow$ & \textbf{RSI} $\uparrow$ & \textbf{HPSv3} $\uparrow$ & \textbf{HPSv2} $\uparrow$ & \textbf{PickScore} $\uparrow$ & \textbf{ImageReward} $\uparrow$ & \textbf{AesScore} $\uparrow$ \\
        \midrule
        % --- FLUX Block ---
        FLUX-Base & 0.417 & 1.00 (Ref.) & 10.307 & 0.303 & 22.797 & 1.037 & 5.793 \\
        FLUX-SFT & 0.391 & 1.03 &  10.320 & 0.303 & 22.808 & 1.097 &  \textbf{5.822} \\
        FLUX-DPO  & 0.293 & 1.13 & 9.68 & 0.299 & 22.476 & 1.062 & 5.752   \\
        \textbf{FLUX-ASAP $(\alpha=0)$} & 0.337 & 1.10 & 10.355 & \textbf{0.306} & 22.806 & \textbf{1.108} & 5.808 \\
        \textbf{FLUX-ASAP $(\alpha=10)$} & \textbf{0.289} & \textbf{1.17} & \textbf{10.360} & 0.304 & \textbf{22.814} & 1.102 & 5.779\\
        \bottomrule
    \end{tabular}
    }
\end{table}

\section{Additional Qualitative Results}
To complement the preliminary visual comparison presented in the main paper, \cref{fig:flux_comparison} and \cref{fig:sdxl_comparison} provide a comprehensive qualitative evaluation of the ASAP framework across both FLUX and SDXL architectures. These extended results demonstrate the generalization of our approach. Specifically, while the unaligned base models frequently struggle with complex hand and facial structures, the ASAP-aligned models consistently improve anatomical plausibility.

\begin{figure}[!t]
  \centering
  \makebox[\textwidth][c]{\includegraphics[width=1.05\linewidth]{ECCV_2026_AnatomyDPO/figures/comparison_flux.pdf}}
  \caption{\textbf{Qualitative Comparison on FLUX.} We showcase visual comparisons between the unaligned FLUX-Base (top row) and our FLUX-ASAP (bottom row). ASAP effectively resolves explicit anatomical artifacts while preserving overall image quality.
  }
  \label{fig:flux_comparison}
\end{figure}

\begin{figure}[!t]
  \centering
  \makebox[\textwidth][c]{\includegraphics[width=1.05\linewidth]{ECCV_2026_AnatomyDPO/figures/comparison_sdxl.pdf}}
  \caption{\textbf{Qualitative results on SDXL.} We showcase visual comparisons between the unaligned SDXL-Base (top row) and our SDXL-ASAP (bottom row). ASAP successfully corrects anatomical artifacts, demonstrating the generalization of our method.
  }
  \label{fig:sdxl_comparison}
\end{figure}

% \clearpage  % TODO FINAL: This \clearpage needs to be removed from both review and camera-ready versions.

%\section*{Acknowledgements}
%Please insert your acknowledgments here.

% ---- Bibliography ----
%
% BibTeX users should specify bibliography style 'splncs04'.
% References will then be sorted and formatted in the correct style.

\clearpage

\bibliographystyle{splncs04}
\bibliography{main}
\end{document}
