# Supplementary material for: Towards Anatomically Plausible Human Image Generation via Synthetic Localized Preferences
Source: arXiv:2605.25759 source file (2026-11-25)
Supplement: Supplementary file 2 [file more_qualitative.tex]

%%%%%%%%%%%%%%%%%%%%%%%%%%%%%%%%%%%%%%%%%%%%%%%%%%%%%%%%%%%%%%%%%%%%%%%%%%%%%%%
% figs_appendix/more_qualitative.tex — 附录大图示例
% 写法提示：附录长图可拆多页，每页一个 figure，各自 label；
%           正文引用 \suppl's~\cref{fig:more_qualitative}。
%%%%%%%%%%%%%%%%%%%%%%%%%%%%%%%%%%%%%%%%%%%%%%%%%%%%%%%%%%%%%%%%%%%%%%%%%%%%%%%

\begin{figure}[t]
    \centering
    \scriptsize
    \begin{tikzpicture}
    % Placeholder figure: replace this tikzpicture with
    % \includegraphics[width=\linewidth]{pdfs/your_figure.pdf}
    \draw[line width=0.6pt, gray!60] (0,0) rectangle (12,3.5);
    \draw[gray!40] (0,0) grid[step=1] (12,3.5);
    \node[gray] at (6,1.75) {\scriptsize Figure placeholder};
\end{tikzpicture}
    \caption{\scriptsize \textbf{Additional Qualitative Comparisons.} Placeholder.}
    \label{fig:more_qualitative}
\end{figure}
