# Supplementary material for: Towards Anatomically Plausible Human Image Generation via Synthetic Localized Preferences
Source: arXiv:2605.25759 source file (2026-11-25)
Supplement: Supplementary file 3 [file extra_ablation.tex]

%%%%%%%%%%%%%%%%%%%%%%%%%%%%%%%%%%%%%%%%%%%%%%%%%%%%%%%%%%%%%%%%%%%%%%%%%%%%%%%
% tabs_appendix/extra_ablation.tex — 附录消融表（占位）
%%%%%%%%%%%%%%%%%%%%%%%%%%%%%%%%%%%%%%%%%%%%%%%%%%%%%%%%%%%%%%%%%%%%%%%%%%%%%%%

\begin{table}[t]
\centering
\renewcommand{\arraystretch}{1.2}
\resizebox{0.7\textwidth}{!}{
\begin{tabular}{l|cc}
\bottomrule
Setting & \down{Chamfer$\downarrow$} & \up{PSNR$\uparrow$} \\ \cline{1-3}
Option 1 & 0.000 & 0.00 \\ \rowcolor{gray!20}
Option 2 (default) & \textbf{0.000} & \textbf{0.00} \\ \toprule
\end{tabular}}
\caption{\textbf{Extra Ablation (Appendix).} Placeholder.}
\label{tab:extra_ablation}
\end{table}
